# Supplementary material for: Consistent machine learning for topology optimization with microstructure-dependent neural network material models
Source: arXiv:2408.13843 source file (2024-08-27)
Supplement: Supplementary file 1 [file appendix-b.tex]

\section{Appendix B}
\label{section:appendix_b}

\emph{Appendix...}
